# Supplementary material for: Derivative-Free Policy Optimization for Linear Risk-Sensitive and Robust Control Design: Implicit Regularization and Sample Complexity
Source: arXiv:2101.01041 source file (2021-12-30)
Supplement: Supplementary file 3 [file Appendix2.tex]

\subsection{Auxiliary Bounds}
Define the following polynomials of $\cG(\bK, \bL(\bK))$:
\small
\begin{align*}
	&c_{1, \bK} := \frac{\cG(\bK, \bL(\bK))}{\phi} + \frac{\|\bD\|^2_F\cG(\bK, \bL(\bK))^2}{\phi^2\cdot\lambda_{\min}(\bH_{\bK, \bL(\bK)})}, \qquad c_{2, \bK} := \sqrt{\frac{\|\bG_{\bK, \bL(\bK)}\|}{\phi}\cdot\big(\cG(\bK, \bL(\bK)) - \cG(\bK^*, \bL^*)\big)}, \\
	&c_{3, \bK} := \frac{c_{2, \bK} + \|\bB\|_F\|\bA\|_Fc_{1, \bK}}{\lambda_{\min}(\bR^u)}, \qquad c_{4, \bK} := \frac{\|\bD\|_F\cG(\bK, \bL(\bK))}{\phi\cdot\lambda_{\min}(\bH_{\bK, \bL(\bK)})} \big(\|\bA\|_F + \|\bB\|_Fc_{3, \bK}\big),\\
	&c_{5, \bK} := 2\Big[\|\bR^u\|_F + \|\bB\|_F^2\cG(\bK, \bL(\bK)) + \|\bB\|_F\|\bD\|_F\cG(\bK, \bL(\bK))\cB_{\bL(\bK), \bK} + \cB_{\bP, \bK}\|\bB\|_F\Big(\|\bB\|_F\big(c_{3, \bK} + \cB_{1, \bK}\big) + \|\bA\|_F + \|\bD\|_F(c_{4, \bK} +\cB_{\bL(\bK), \bK})\Big)\Big],
\end{align*}
\normalsize
where $\cB_{1, \bK}, \cB_{\bP, \bK}, \cB_{\bL(\bK), \bK}$ follows from Lemma \ref{lemma:outer_perturb} and $\bG_{\bK, \bL}$ is defined in \eqref{eqn:gh_def}. Then, we present the following lemmas.

\begin{lemma} For $\bK, \bK' \in \cK$, the following inequalities hold
\vspace{-2em}
\begin{flushleft}
\begin{minipage}[t]{0.33\textwidth}
\begin{align}
	&\|\bP_{\bK, \bL(\bK)}\|_F \leq \cG(\bK, \bL(\bK))/\phi \label{bound:pk}, \\
	&\|\tilde{\bP}_{\bK, \bL(\bK)}\|_F \leq c_{1, \bK} \label{bound:tilde_pk},
\end{align}
\end{minipage}
\begin{minipage}[t]{0.39\textwidth}
\begin{align}
&\|\bF_{\bK, \bL(\bK)}\|_F \leq c_{2, \bK} \label{bound:fk} \\
 &\|\nabla_{\bK}\cG(\bK, \bL(\bK))\|_F \leq 2\|\Sigma_{\bK, \bL(\bK)}\|c_{2, \bK},\label{bound:grad_K}
\end{align}
\end{minipage}
\begin{minipage}[t]{0.27\textwidth}
\begin{align}
 	&\|\bK\|_F \leq c_{3, \bK} \label{bound:k}, \\ 
	&\|\bL(\bK)\|_F \leq c_{4, \bK}. \label{bound:lk}	
\end{align}
\end{minipage}
\end{flushleft}
\end{lemma}

\begin{proof}
To start with, we note that for any $\bK \in \cK$, the solution to the Riccati equation \eqref{eqn:DARE_black_L} satisfies $\bP_{\bK,\bL(\bK)}\geq 0$. Thus, \eqref{bound:pk} can be proved by $\cG(\bK, \bL(\bK)) = \Tr(\bP_{\bK, \bL(\bK)}\Sigma_0) \geq \phi\|\bP_{\bK, \bL(\bK)}\|_F$, where the inequality follows from $\phi = \lambda_{\min}(\Sigma_0) >0$ and $\Tr(M) \geq \|M\|_F$ for any matrix $M \geq 0$. Then, for any $\bK \in \cK$, we have by \eqref{bound:pk} and the definition of $\tilde{\bP}_{\bK, \bL(\bK)}$ in \eqref{eqn:tilde_pk} that
\begin{align*}
	\big\|\tilde{\bP}_{\bK, \bL(\bK)}\big\|_F &\leq \big\|\bP_{\bK, \bL(\bK)}\big\|_F + \big\|\bP_{\bK, \bL(\bK)}\bD\bH_{\bK, \bL(\bK)}^{-1}\bD^{\top}\bP_{\bK, \bL(\bK)}\big\|_F \leq \frac{\cG(\bK, \bL(\bK))}{\phi} + \frac{\|\bD\|^2_F\cG(\bK, \bL(\bK))^2}{\phi^2\cdot\lambda_{\min}(\bH_{\bK, \bL(\bK)})} = c_{1, \bK}.
\end{align*}
This completes the proof of \eqref{bound:tilde_pk}. Subsequently, for any $\bK, \bK' \in \cK$, we invoke Lemma 11 of \cite{fazel2018global} to get 
	\begin{align*}
	\cG(\bK, \bL(\bK)) - \cG(\bK^*, \bL^*) &\geq \cG(\bK, \bL(\bK)) - \cG(\bK', \bL(\bK')) \geq \frac{\phi}{\|\bG_{\bK, \bL(\bK)}\|}\Tr(\bF_{\bK, \bL(\bK)}^{\top}\bF_{\bK, \bL(\bK)}).
	\end{align*}
	As a result,  we have $\|\bF_{\bK, \bL(\bK)}\|^2_F = \Tr(\bF_{\bK, \bL(\bK)}^{\top}\bF_{\bK, \bL(\bK)})\leq \frac{\|\bG_{\bK, \bL(\bK)}\|}{\phi} \big(\cG(\bK, \bL(\bK)) - \cG(\bK^*, \bL^*)\big)$, and taking a square root of both sides yields \eqref{bound:fk}. Moreover, we can prove \eqref{bound:grad_K} such that
	\begin{align*}
		\|\nabla_{\bK}\cG(\bK, \bL(\bK))\|_F^2 \leq 4\|\Sigma_{\bK, \bL(\bK)}\|^2\Tr(\bF_{\bK, \bL(\bK)}^{\top}\bF_{\bK, \bL(\bK)}) \leq \frac{4\|\Sigma_{\bK, \bL(\bK)}\|^2\|\bG_{\bK, \bL(\bK)}\|}{\phi} \big(\cG(\bK, \bL(\bK)) - \cG(\bK^*, \bL(\bK^*))\big).
	\end{align*}
	Next, we invoke Lemma 25 of \cite{fazel2018global} and \eqref{bound:tilde_pk} to get
 	\begin{align*}
 		\|\bK\|_F &\leq \frac{c_{2, \bK}}{\lambda_{\min}(\bR^u)}+ \frac{\big\|\bB^{\top}\tilde{\bP}_{\bK, \bL(\bK)}\bA\big\|_F}{\lambda_{\min}(\bR^u)} \leq \frac{c_{2, \bK} + \|\bB\|_F\|\bA\|_Fc_{1, \bK}}{\lambda_{\min}(\bR^u)} = c_{3, \bK},
 \end{align*}
 which proves \eqref{bound:k}. Lastly, for any $\bK \in \cK$ and recall the definition of $\bL(\bK)$ from \eqref{eqn:l_k}
\begin{align*}
	\|\bL(\bK)\|_F = \|\bH_{\bK, \bL(\bK)}^{-1}\bD^{\top}\bP_{\bK, \bL(\bK)}(\bA-\bB\bK)\|_F \leq \frac{\|\bD\|_F\cG(\bK, \bL(\bK))}{\phi\cdot\lambda_{\min}(\bH_{\bK, \bL(\bK)})} \big(\|\bA\|_F + \|\bB\|_Fc_{3, \bK}\big) = c_{4, \bK},
\end{align*}
which proves \eqref{bound:lk}. 
\end{proof}

\begin{lemma}\label{lemma:subfk}
	For $\bK, \bK' \in \cK$ satisfying $\|\bK' - \bK\|_F \leq \cB_{1, \bK}$, where $\cB_{1, \bK}$ is as defined in Lemma \ref{lemma:outer_perturb}, it holds that
	\begin{align}
	 \|\bF_{\bK', \bL(\bK')} - \bF_{\bK, \bL(\bK)}\|_F \leq c_{5, \bK}\cdot \|\bK'-\bK\|_F. \label{bound:subfk}	
	\end{align}
\end{lemma}
\begin{proof}
For $\bK, \bK' \in \cK$ and recalling the definition of $\bF_{\bK, \bL}$ in \eqref{eqn:nabla_K}, we have
\small
\begin{align*}
	&\hspace{-1em}\|\bF_{\bK', \bL(\bK')} - \bF_{\bK, \bL(\bK)}\|_F = 2\big\|(\bR^u + \bB^{\top}\bP_{\bK', \bL(\bK')}\bB)\bK' - \bB^{\top}\bP_{\bK', \bL(\bK')}(\bA-\bD\bL(\bK')) - (\bR^u + \bB^{\top}\bP_{\bK, \bL(\bK)}\bB)\bK - \bB^{\top}\bP_{\bK, \bL(\bK)}(\bA-\bD\bL(\bK))\big\|_F\\
	&\leq 2\|\bR^u\|_F\|\bK'-\bK\|_F + 2\|\bB\|_F^2\|\bK'\|_F\|\bP_{\bK', \bL(\bK')}- \bP_{\bK, \bL(\bK)}\|_F + 2\|\bB\|^2_F\|\bP_{\bK, \bL(\bK)}\|_F\|\bK'-\bK\|_F + 2\|\bB\|_F\|\bA\|_F\|\bP_{\bK', \bL(\bK')}- \bP_{\bK, \bL(\bK)}\|_F\\
	&\hspace{1em}  + 2\|\bB\|_F\|\bD\|_F\|\bL(\bK')\|_F\|\bP_{\bK', \bL(\bK')}- \bP_{\bK, \bL(\bK)}\|_F + 2\|\bB\|_F\|\bP_{\bK, \bL(\bK)}\|_F\|\bD\|_F\|\bL(\bK') - \bL(\bK)\|_F\\
	&= 2\big(\|\bR^u\|_F + \|\bB\|^2_F\|\bP_{\bK, \bL(\bK)}\|_F\big)\cdot \|\bK'-\bK\|_F + 2\big(\|\bB\|_F\|\bP_{\bK, \bL(\bK)}\|_F\|\bD\|_F\big)\cdot\|\bL(\bK') - \bL(\bK)\|_F\\
	&\hspace{1em}+ 2\Big(\|\bB\|^2_F\big(\|\bK\|_F + \|\bK'-\bK\|_F\big) + \|\bB\|_F\|\bA\|_F + \|\bB\|_F\|\bD\|_F\big(\|\bL(\bK)\|_F+ \|\bL(\bK') -\bL(\bK)\|_F\big)\Big)\cdot \|\bP_{\bK', \bL(\bK')} - \bP_{\bK, \bL(\bK)}\|_F.
\end{align*}
\normalsize
Applying \eqref{bound:pk}, \eqref{bound:k}, \eqref{bound:lk}, \eqref{eqn:p_perturb}, and \eqref{eqn:lk_perturb} proves \eqref{bound:subfk}, such that
\begin{align*}
	\|\bF_{\bK', \bL(\bK')} - \bF_{\bK, \bL(\bK)}\|_F &\leq 2\big(\|\bR^u\|_F+ \|\bB\|^2_F\cG(\bK, \bL(\bK))\big)\cdot \|\bK'-\bK\|_F + 2\big(\|\bB\|_F\|\bD\|_F\cG(\bK, \bL(\bK))\big)\cdot\|\bL(\bK') - \bL(\bK)\|_F \\
	&\hspace{1em} + 2\Big(\|\bB\|_F^2\big(c_{3, \bK} + \cB_{1, \bK}\big) + \|\bB\|_F\|\bA\|_F + \|\bB\|_F\|\bD\|_F(c_{4, \bK}+\cB_{\bL(\bK), \bK})\Big)\cdot \|\bP_{\bK', \bL(\bK')} - \bP_{\bK, \bL(\bK)}\|_F\\
	&\leq 2\Big[\|\bR^u\|_F + \|\bB\|_F^2\cG(\bK, \bL(\bK)) + \|\bB\|_F\|\bD\|_F\cG(\bK, \bL(\bK))\cB_{\bL(\bK), \bK} \\
	&\hspace{1em} + \cB_{\bP, \bK}\|\bB\|_F\Big(\|\bB\|_F\big(c_{3, \bK} + \cB_{1, \bK}\big) + \|\bA\|_F + \|\bD\|_F(c_{4, \bK} +\cB_{\bL(\bK), \bK})\Big)\Big] \cdot \|\bK'-\bK\|_F.
\end{align*}
This completes the proof.
\end{proof}
